# Supplementary material for: Abstraction Logic: The Marriage of Contextual Refinement and Separation Logic
Source: arXiv:2109.02991 source file (2021-09-07)
Supplement: Supplementary file 1 [file appendix.tex]

\section{Appendix}
\label{sec:appendix}

Text of appendix \ldots

%%% Local Variables:
%%% mode: latex
%%% TeX-master: "main"
%%% End:
